# Supplementary material for: Iterative Mode-Dropping for the Sum Capacity of MIMO-MAC with Per-Antenna Power Constraint
Source: arXiv:1202.0445 source file (2012-02-02)
Supplement: Supplementary file 1 [file Appendix.tex]

\appendices
% you can choose not to have a title for an appendix
% if you want by leaving the argument blank
\section{Proof of Convergence Behavior}
\label{appendix:PCB}
In this appendix, we prove the convergence behavior of the algorithm, which states that the sum rate is at most $(K-1)m/2$ nats away from the sum capacity after one iteration. 
The problem in (\ref{perantennapowerMAC}) can be rewritten as
\begin{IEEEeqnarray}{rCl}
\label{primary} 
\max \quad&&\log |\mathbf{T}| \nonumber \\
\text{s.t.} \quad&&\mathbf{T}\preccurlyeq \mathbf{I}_m+\sum_{i=1}^{K}\mathbf{H}_{i}\mathbf{Q}_{i}\mathbf{H}_{i}^{\dagger}\nonumber\\
&&\text{diag}(\mathbf{Q}_i) \preccurlyeq \mathbf{P}_i \quad i=1,\cdots,K\nonumber \\
&&\mathbf{Q}_i \succcurlyeq 0,\quad \quad \quad\quad i=1,\cdots,K \;.
\end{IEEEeqnarray}
The Lagrangian of the above problem becomes
\begin{IEEEeqnarray}{rCl}
\label{multiLagrangiannew} 
\mathcal{L}(\mathbf{Q}_i, \mathbf{T}, \mathbf{\Gamma}, \mathbf{D}_i,\mathbf{M}_i)\hspace{-65pt}&& \nonumber\\
&=&-\log |\mathbf{T}|+\text{tr}\left[\mathbf{\Gamma}\left(\mathbf{T}-\sum_{i=1}^{K}\mathbf{H}_i\mathbf{Q}_i\mathbf{H}_{i}^{\dagger}\right)\right] \nonumber \\
&&{}- \sum_{i=1}^{K}\text{tr}[{(\mathbf{D}_i(\mathbf{Q}_i-\mathbf{P}_i)}]+\sum_{i=1}^{K}\text{tr}(\mathbf{M}_i\mathbf{Q}_i)\nonumber\\
&=&-\log |\mathbf{T}|+\text{tr}(\mathbf{\Gamma T})-\text{tr}(\mathbf{\Gamma}) -\sum_{i=1}^{K}\text{tr}(\mathbf{D}_i\mathbf{P}_i)\nonumber\\
&&{}+\sum_{i=1}^{K}\text{tr}\left[\left(\mathbf{D}_i-\mathbf{H}_i^{\dagger}\mathbf{\Gamma}\mathbf{H}_{i}-\mathbf{M}_i\right)\mathbf{Q}_i\right]\;,
\end{IEEEeqnarray}
where $\mathbf{\Gamma}$ is the dual variable associated with the first positive semidefinite constraints in the primal and is positive semidefinite, $\mathbf{M}_i$'s are dual variables with last $K$ positive semidefinite constraints and are positive semidefinite and $\mathbf{D}_i$'s are the dual variables corresponding to the per-antenna power constraint and are all diagonal matrix.
The objective function of dual is expressed as
\begin{IEEEeqnarray}{rCl}
\label{dualobject} 
{q}(\mathbf{\Gamma}, \mathbf{D}_i,\mathbf{M}_i)=\inf_{\mathbf{Q}_i,\mathbf{T}}\mathcal{L}(\mathbf{Q}_i, \mathbf{T}, \mathbf{\Gamma}, \mathbf{D}_i,\mathbf{M}_i)\;.
\end{IEEEeqnarray}
Take the derivative of $\mathcal{L}$ with respect to $\mathbf{Q}_i$ and $\mathbf{T}$, we obtain
\begin{IEEEeqnarray}{rCl}
\label{dualderiavative} 
&&\mathbf{D}_i=\mathbf{H}_i^{\dagger}\mathbf{\Gamma}\mathbf{H}_i+\mathbf{M}_i, \quad i=1,2\cdots, K \\
&&\mathbf{\Gamma}=\mathbf{T}^{-1}\;.
\end{IEEEeqnarray}
The dual of the this problem is shown as follows,
\begin{IEEEeqnarray}{rCl}
\label{dual} 
\min \quad&&\log |\mathbf{\Gamma}|+m-\text{tr}(\mathbf{\Gamma})-\sum_{i=1}^K\text{tr}(\mathbf{D}_i\mathbf{P}_i) \nonumber \\
\text{s.t.} \quad &&\mathbf{D}_i \succcurlyeq \mathbf{H}_{i}^{\dagger}\mathbf{\Gamma}\mathbf{H}_{i},\quad i=1,2,\cdots,K \nonumber\\
&&\mathbf{\Gamma} \succcurlyeq 0 \;,
\end{IEEEeqnarray}
where the first constraint results from the positive semidefinite property of the dual variable $\mathbf{M}_i$'s. 

The duality gap $d$ is the difference between the objective functions of primal and dual, read as
\begin{IEEEeqnarray}{rCl}
\label{dualitygap} 
d=\text{tr}\left(\sum_{i=1}^{K}\mathbf{H}_i\mathbf{Q}_i\mathbf{H}_{i}^{\dagger}+\mathbf{I}_m\right)^{-1}+\sum_{i=1}^{K}\text{tr}(\mathbf{D}_i\mathbf{P}_i)-m \;.\qquad 
\end{IEEEeqnarray}
To make the duality gap tight, $\mathbf{D}_i$ is chosen to be the solution of optimization problem, as follows,
\begin{IEEEeqnarray}{rCl}
\label{D_iOptimization} 
\min \quad&&\text{tr}(\mathbf{D}_i\mathbf{P}_i)\nonumber \\
\text{s.t.} \quad &&\mathbf{D}_i \succcurlyeq \mathbf{H}_{i}^{\dagger}\left(\sum_{i=1}^{K}\mathbf{H}_i\mathbf{Q}_i\mathbf{H}_{i}^{\dagger}+\mathbf{I}_m\right)^{-1}\mathbf{H}_{i}\quad \;.
\end{IEEEeqnarray}

At the beginning of the algorithm, all covariance matrix are initialized to be 0 at the beginning. Therefore, in the first iteration, for each user the covariance matrix is optimized using single-user mode-dropping by treating the interference from previous users as noise. For $i$th user, duality gap can be zero as the single-user mode-dropping converges. Therefore, we have
\begin{IEEEeqnarray}{rCl}
\label{dualitygapuseri} 
\text{tr}\left[\left(\sum_{i=1}^{i}\mathbf{H}_i\mathbf{Q}_i\mathbf{H}_{i}^{\dagger}+\mathbf{I}_m\right)^{-1}\left(\sum_{i=1}^{i-1}\mathbf{H}_i\mathbf{Q}_i\mathbf{H}_{i}^{\dagger}+\mathbf{I}_m\right)\right]\qquad \quad\nonumber \\
{}+\text{tr}(\mathbf{D}'_i\mathbf{P}_i)-m=0 \;, \qquad 
\end{IEEEeqnarray}
where $\mathbf{D}'_i$ is chosen to be the solution of the following optimization problem
\begin{IEEEeqnarray}{rCl}
\label{D_i'Optimization} 
\min \quad&&\text{tr}(\mathbf{D}'_i\mathbf{P}_i)\nonumber \\
\text{s.t.} \quad &&\mathbf{D}'_i \succcurlyeq \mathbf{H}_{i}^{\dagger}\left(\sum_{i=1}^{i}\mathbf{H}_i\mathbf{Q}_i\mathbf{H}_{i}^{\dagger}+\mathbf{I}_m\right)^{-1}\mathbf{H}_{i}\;.\quad  
\end{IEEEeqnarray}
%Collectively, all $\mathbf{D}'_i$'s are the solutions of the problem, read as
%\begin{IEEEeqnarray}{rCl}
%\label{D_i'sOptimization} 
%\min \quad&&\sum_{i=1}^{K}\text{tr}(\mathbf{D}'_i\mathbf{P}_i)\nonumber \\
%\text{s.t.} \quad &&\mathbf{D}'_i \succcurlyeq \mathbf{H}_{i}^{\dagger}\left(\sum_{i=1}^{i}\mathbf{H}_i\mathbf{Q}_i\mathbf{H}_{i}^{\dagger}+\mathbf{I}_m\right)^{-1}\mathbf{H}_{i}\quad  
%\nonumber \\ 
%&&\qquad \qquad \qquad \qquad \quad  i=1,2,\cdots,K \quad
%\end{IEEEeqnarray}
Since
\begin{IEEEeqnarray}{rCl}
\label{Hinequality} 
\mathbf{H}_{i}^{\dagger}\left(\sum_{i=1}^{K}\mathbf{H}_i\mathbf{Q}_i\mathbf{H}_{i}^{\dagger}+\mathbf{I}_m\right)^{-1}\mathbf{H}_{i}\qquad \qquad \qquad \qquad \quad\nonumber\\  
\preccurlyeq \mathbf{H}_{i}^{\dagger}\left(\sum_{i=1}^{i}\mathbf{H}_i\mathbf{Q}_i\mathbf{H}_{i}^{\dagger}+\mathbf{I}_m\right)^{-1}\mathbf{H}_{i}\nonumber\\ \qquad \qquad \qquad \qquad \quad  i=1,2,\cdots,K\;, \quad 
\end{IEEEeqnarray}
the feasible region of optimization problem (\ref{D_iOptimization}) is no smaller than that in (\ref{D_i'Optimization}), thus at the optimum,
\begin{IEEEeqnarray}{rCl}
\label{Dinequality} 
\text{tr}(\mathbf{D}_i\mathbf{P_i})\preccurlyeq \text{tr}(\mathbf{D}'_i\mathbf{P_i}),  \quad \quad i=1,2,\cdots,K\;. \quad 
\end{IEEEeqnarray}
Since $\text{tr}(\mathbf{A}) \preccurlyeq \text{tr}(\mathbf{B})$ can follows from $\mathbf{A} \preccurlyeq \mathbf{B}$,
\begin{IEEEeqnarray}{rCl}
\label{suminequality} 
\text{tr}\left(\sum_{i=1}^{K}\mathbf{H}_i\mathbf{Q}_i\mathbf{H}_{i}^{\dagger}+\mathbf{I}_m\right)^{-1} \preccurlyeq \text{tr}\left(\mathbf{H}_1\mathbf{Q}_1\mathbf{H}_{1}^{\dagger}+\mathbf{I}_m\right)^{-1}\;.
\end{IEEEeqnarray}
Since $\text{tr}(\mathbf{AB})=\text{tr}(\mathbf{BA})$ and the trace of a positive semidefinite matrix is positive,
if define $\mathbf{C}=\left(\sum_{i=1}^{i-1}\mathbf{H}_i\mathbf{Q}_i\mathbf{H}_{i}^{\dagger}+\mathbf{I}_m\right)$, we obtain
\begin{IEEEeqnarray}{rCl}
\label{traceinequality} 
\text{tr}\left[\left(\sum_{i=1}^{i}\mathbf{H}_i\mathbf{Q}_i\mathbf{H}_{i}^{\dagger}+\mathbf{I}_m\right)^{-1}\mathbf{C}\right]\qquad \qquad \qquad \quad\nonumber\\
=\text{tr}\left[\mathbf{C}^{1/2}\left(\sum_{i=1}^{i}\mathbf{H}_i\mathbf{Q}_i\mathbf{H}_{i}^{\dagger}+\mathbf{I}_m\right)^{-1}\mathbf{C}^{1/2}\right] >0\;.
\end{IEEEeqnarray}
Hence we have
\begin{IEEEeqnarray}{rCl}
\label{minequality} 
\text{tr}(\mathbf{D}'_i\mathbf{P}_i)\leq m, \quad \quad i=1,2,\cdots,K\;. \quad
\end{IEEEeqnarray}
The duality gap can be bounded as below
\begin{IEEEeqnarray}{rCl}
\label{dualitygapbounded} 
d&=&\text{tr}\left(\sum_{i=1}^{K}\mathbf{H}_i\mathbf{Q}_i\mathbf{H}_{i}^{\dagger}+\mathbf{I}_m\right)^{-1}+\sum_{i=1}^{K}\text{tr}(\mathbf{D}_i\mathbf{P}_i)-m \nonumber \\
&\leq&\text{tr}\left(\sum_{i=1}^{K}\mathbf{H}_i\mathbf{Q}_i\mathbf{H}_{i}^{\dagger}+\mathbf{I}_m\right)^{-1}+\sum_{i=1}^{K}\text{tr}(\mathbf{D}'_i\mathbf{P}_i)-m \nonumber \\
&=&\text{tr}\left(\sum_{i=1}^{K}\mathbf{H}_i\mathbf{Q}_i\mathbf{H}_{i}^{\dagger}+\mathbf{I}_m\right)^{-1}+\text{tr}(\mathbf{D}_1\mathbf{P}_1)-m+\sum_{i=2}^{K}\text{tr}(\mathbf{D}'_i\mathbf{P}_i) \nonumber \\
&\leq&\text{tr}\left(\mathbf{H}_1\mathbf{Q}_1\mathbf{H}_{1}^{\dagger}+\mathbf{I}_m\right)^{-1}+\text{tr}(\mathbf{D}_1\mathbf{P}_1)-m+\sum_{i=2}^{K}\text{tr}(\mathbf{D}'_i\mathbf{P}_i) \nonumber\\
&=&\sum_{i=2}^{K}\text{tr}(\mathbf{D}'_i\mathbf{P}_i) \nonumber\\
&\leq&m(K-1) \;.\nonumber
\end{IEEEeqnarray}
where the first inequalities follows from (\ref{Dinequality}), the second inequalities follows from (\ref{suminequality}), the third inequality follows from (\ref{minequality}) and the last equality follows from (\ref{dualitygapuseri}) when $i$ is set to be $1$. Here we complete the proof.
